# Supplementary material for: An all-magnonic neuron with tunable fading memory
Source: arXiv:2509.18321 ancillary file (2026-03-04)
Supplement: Supplementary file 1 [file 20250922_Suppl_All-magnonic-Neuron.pdf]

# Supplemental Material - All-magnonic neurons for analog artificial neural networks

David Breitbach<sup>1\*</sup>, Moritz Bechberger<sup>1†</sup>, Hanadi Mortada<sup>1</sup>,  
Björn Heinz<sup>1</sup>, Roman Verba<sup>2</sup>, Qi Wang<sup>3</sup>, Carsten Dubs<sup>4</sup>,  
Mario Carpentieri<sup>5</sup>, Giovanni Finocchio<sup>6</sup>, Davi Rodrigues<sup>5</sup>,  
Alexandre Abbass Hamadeh<sup>7</sup>, Philipp Pirro<sup>1</sup>

<sup>1\*</sup>Fachbereich Physik and Landesforschungszentrum OPTIMAS, RPTU  
Kaiserslautern-Landau, Kaiserslautern, 67663, Germany.

<sup>2</sup>V. G. Baryakhtar Institute of Magnetism of the NAS of Ukraine, Kyiv,  
03142, Ukraine.

<sup>3</sup>School of Physics, Hubei Key Laboratory of Gravitation and Quantum  
Physics, Institute for Quantum Science and Engineering, Huazhong  
University of Science and Technology, Wuhan, China.

<sup>4</sup>INNOVENT e.V. Technologieentwicklung, Jena, 07745, Germany.

<sup>5</sup>Department of Electrical and Information Engineering, Politecnico di  
Bari, Bari, 70125, Italy.

<sup>6</sup>Department of Mathematical and Computer Sciences, Physical Sciences  
and Earth Sciences, University of Messina, Messina, 98166, Italy.

<sup>7</sup>Centre de Nanosciences et de Nanotechnologies, Université  
Paris-Saclay, Palaiseau, 91120, France.

\*Corresponding author(s). E-mail(s): [dbreitba@rptu.de](mailto:dbreitba@rptu.de);

<sup>†</sup>These authors contributed equally to this work.

## Contents

|   |                                    |   |
|---|------------------------------------|---|
| 1 | Nonlinear magnonic frequency shift | 3 |
| 2 | Numerical neuron model             | 4 |
| 3 | Magnon lifetime and decay length   | 5 |
| 4 | Fading memory                      | 6 |
| 5 | Intrinsic signal accumulation      | 7 |
| 6 | Waveguide neuron bistable foldover | 8 |
| 7 | Non-reciprocal neuron output       | 9 |

# 1 Nonlinear magnonic frequency shift

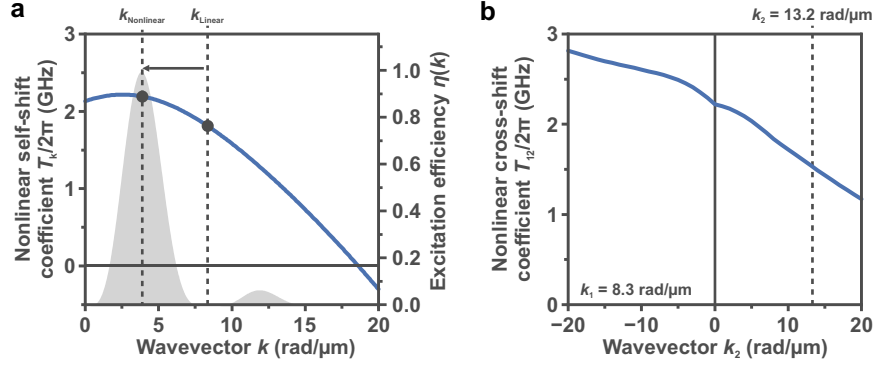

**Fig. S1 | Nonlinear magnonic shift coefficients.** **a** Calculation of the nonlinear magnonic self-shift coefficient  $T_k$  as a function of the magnon wavevector  $k$ . The sub-threshold excitation (linear case) is indicated by  $k_{\text{Linear}}$ , while the point of maximum excitation efficiency is indicated by  $k_{\text{Nonlinear}}$ . **b** Calculation of the nonlinear magnonic cross-shift coefficient  $T_{12}$  for a fixed wavevector  $k_1 = 8.3 \text{ rad } \mu\text{m}^{-1}$ , which corresponds to the pump frequency  $f_1 = 1.69 \text{ GHz}$  in the linear dispersion case. The wavevector of the trigger signal at  $f_2 = 2.2 \text{ GHz}$  is marked by a dashed line at  $k_2 = 13.2 \text{ rad } \mu\text{m}^{-1}$ . Note that both the self- and cross-shift coefficients are positive over a wide wavevector range compared to the regime of neuron operation.

## 2 Numerical neuron model

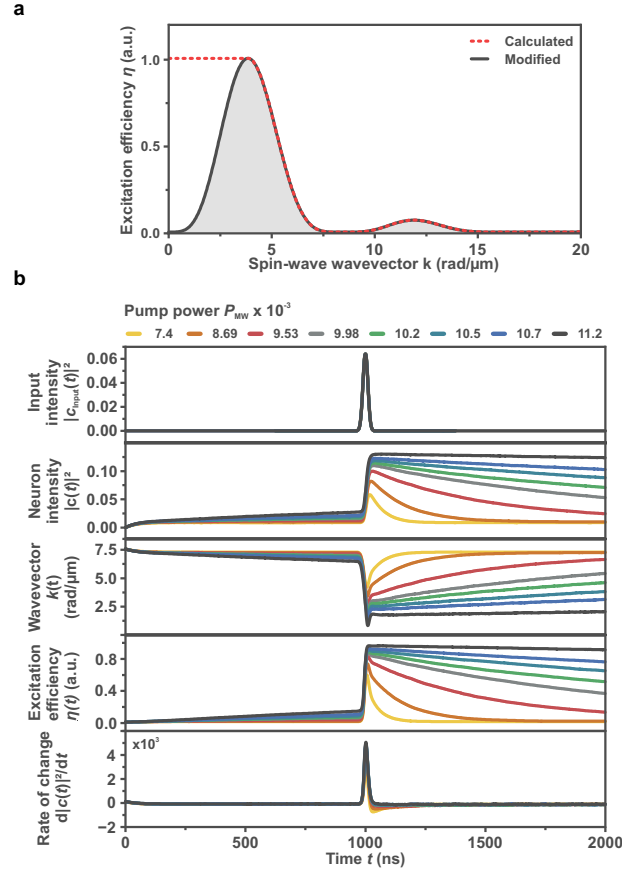

**Fig. S2 | Numerical neuron model.** **a** Linear case calculation of the excitation efficiency  $\eta(k)$  (grey), and modified nonlinear case (red) (see Methods). **b** Additional data on the numerical model results from Fig. 3d (main text). **First panel:** Gaussian-shaped neuron input intensity  $|c_{\text{in}}(t)|^2$ . **Second panel:** The neuron output intensity  $|c_{\text{neu}}(t)|^2$  shows, after an equilibration time, a significant increase during the trigger pulse, followed by a decay process which depends on the pump power  $P_{\text{MW}}$ . Note that the input intensity  $|c_{\text{in}}(t)|^2$  is smaller than the neuron intensity  $|c_{\text{neu}}(t)|^2$ , showing that a significant part of the neuron activation intensity is contributed by the neuron pump itself. Note that the intensity scaling is given by the nonlinear shift coefficients, which relate absolute magnon intensity and frequency shift in GHz. For comparison with BLS data, a scaling with offset was applied (see Methods). **Third panel:** The excited magnon wavevector  $k(t)$  upon neuron activation, before decaying back to the equilibrium state. **Fourth panel:** The excitation efficiency  $\eta(t)$  as a function of time, showing a significant increase when the neuron is triggered. **Fifth panel:** Rate of change of the neuron intensity  $d|c_{\text{neu}}(t)|^2/dt$  (left side of Eq. (12) in main text) as a function of time. The rate spikes positively during the neuron triggering, followed by a negative rate in the decay process.

### 3 Magnon lifetime and decay length

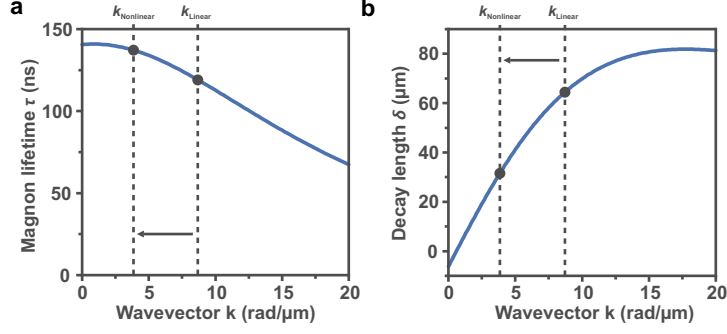

**Fig. S3 | Magnon lifetime and decay length.** **a** Magnon lifetime as a function of the wavevector  $k$ , calculated by  $\tau = (2\pi\alpha A_k)^{-1}$  (see also Methods). This lifetime represents an upper limit to the real lifetime, as it neglects non-Gilbert-like damping mechanisms and, in the case of the waveguide, effects of nanofabrication [1]. **b** The wavevector  $k$  influences not only the lifetime  $\tau$ , but also the group velocity  $v_g$ . As a result, the magnon decay length  $\delta = v_g(k) \cdot \tau(k)$  shown here is also a function of the wavevector  $k$ . Despite the decreasing lifetime, the decay length significantly increases with increasing wavevector  $k$ . This is a result of the quadratic shape of the magnon dispersion relation, reflecting in a strong increase in group velocity  $v_g$  towards higher wavevectors  $k$  (see also Ref. [2]). In the wavevector regime relevant to this work, the magnon decay length is within the range of several tens of micrometers.

## 4 Fading memory

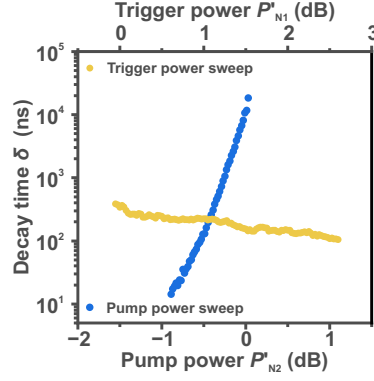

**Fig. S4 | Fading memory time of the activated neuron.** Shown are the fading memory (decay) times extracted from exponential decay fits to Fig. 3 (b) and (d) (main text) as a function of the pump power  $P'_{N2}$  (blue curve, bottom axis) and the trigger power  $P'_{N1}$  (yellow curve, top axis). Note that the bottom and top scales cover the same power interval. While a change of the pump power drastically changes the fading memory time, the trigger power has a comparably slight effect. With increasing trigger power, the fading memory time is reduced. This is most probably attributed to a higher instantaneous amplitude of the neuron after the stronger trigger pulse and, consequently, a stronger contribution of nonlinear scattering and dissipation to the thermalization process.

## 5 Intrinsic signal accumulation

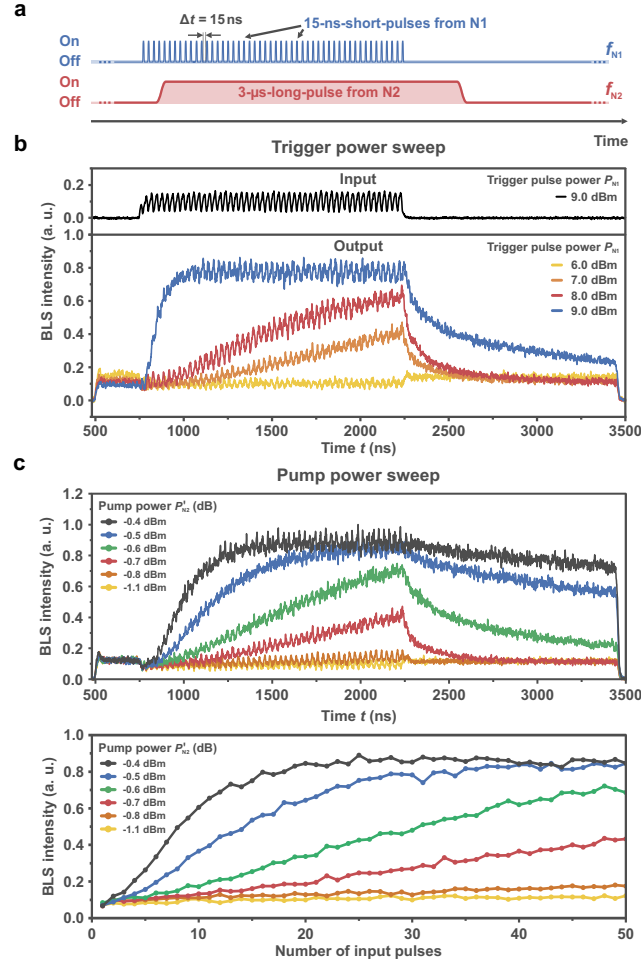

**Fig. S5 | Intrinsic signal accumulation over multiple consecutive input pulses.**

**a** Schematic of pulses applied to the triangular neuron structure: 50 trigger pulses (of 15 ns duration each and a pulse spacing of 15 ns between two consecutive pulses) are excited from neuron **N1** at the frequency  $f_{N1} = 2.2$  GHz and one 3- $\mu$ s-long pump pulse is applied to neuron **N2** at the frequency  $f_{N2} = 1.69$  GHz. **b** Sweep of the input trigger power: Shown is the BLS intensity of the input pulse train (measured before reaching neuron **N2**) as a function of time, as well as the BLS intensity of the output of the triggered neuron **N2** as a function of time for different trigger pulse powers  $P_{N1}$  at a fixed pump power of  $P'_{N2} = -0.7$  dB. **c** Sweep of the pump power: Upper graph - BLS intensity as a function of time for different pump powers  $P'_{N2}$  at a fixed trigger power of  $P_{N1} = 7.0$  dBm. Note that the fading memory time after the trigger pulse train changes with the pump power, while it was almost independent of the trigger power in panel (b). Lower graph - BLS intensity extracted at the temporal positions of the input pulses from the upper graph, and plotted as a function of the number of the input pulse. At low powers, a linear integration regime is established, where the BLS intensity is proportional to the number of integrated pulses, while at higher powers, saturation sets in after a number of pulses.

## 6 Waveguide neuron bistable foldover

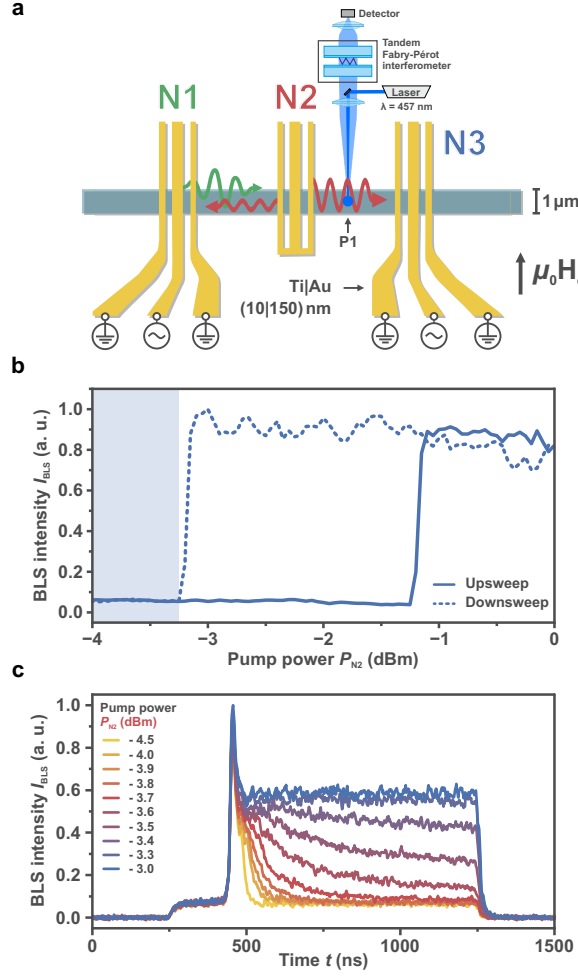

**Fig. S6 | Neuron activation with bistability.** **a** Experiment schematic: Measurement is performed behind neuron **N2** in position P1. Neuron **N2** is pumped, either continuously (**b**), or by a  $1 \mu\text{s}$  pulse (**c**). Neuron **N1** can be used for triggering (**c**). **b** Continuous pumping of neuron **N2** results in a nonlinear step as a function of the pump power  $P_{N2}$  due to the foldover effect. Up- and downsweep of the power reveals a bistability window, i.e., two intensity states can be stabilized at the same powers depending on the history of the system. Applying a power in the bistability window enables another mode of operation of the neuron, where it remains activated after triggering. Neuron operation with autonomous decay or fading memory is still possible if the pump power is chosen below the hysteresis window (blue shaded area), see (**c**). **c** Neuron activation by a  $1\text{-}\mu\text{s}$ -long trigger pulse from **N1** with a  $1\text{-}\mu\text{s}$ -long pump pulse in neuron **N2** of varying pump power. If the pump power is chosen below the bistability window  $P_{N2} < -3.3 \text{ dBm}$ , the neuron decays back to its initial state. For powers  $P_{N2} \geq -3.3 \text{ dBm}$ , the high intensity state can permanently be stabilized and no decay is observed. Note that the spike in the onset of the activation is due to the trigger pulse of **N1**, which is also detected behind **N2**. Trigger pulse power:  $P_{N1} = 0.0 \text{ dBm}$ .



## 7 Non-reciprocal neuron output

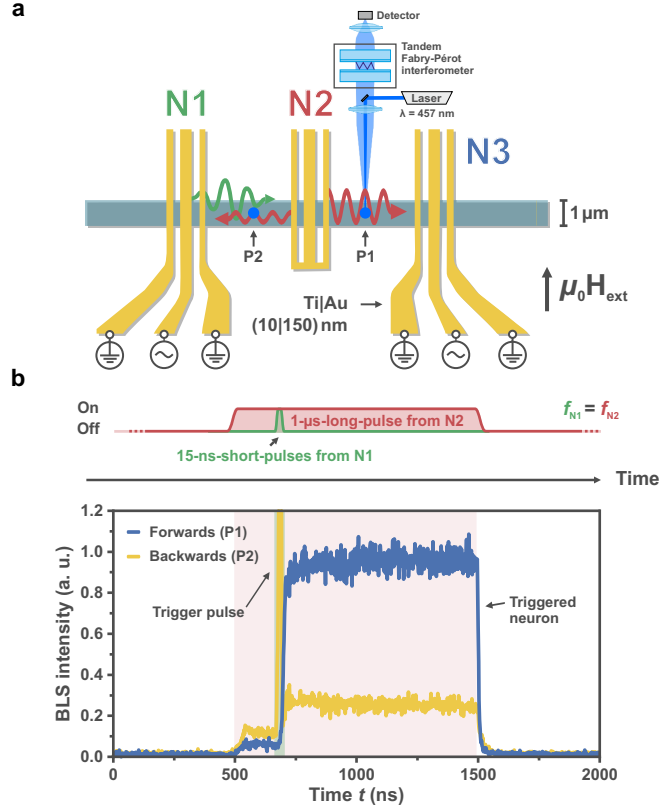

**Fig. S7 | Nonreciprocity of neuron emission.** **a** Schematic of the experiment: A measurement is performed on the waveguide on both sides of neuron **N2**, which is triggered by neuron **N1**. P1 and P2 indicate the measurement positions. **b** Upper panel: Scheme of the applied RF-pulses. A 1- $\mu\text{s}$ -long pump pulse is applied to neuron **N2**, while a 15-ns-short trigger pulse is applied to neuron **N1**. The powers chosen are  $P_{N1} = -2 \text{ dBm}$  and  $P_{N2} = -0.55 \text{ dBm}$ , which are not comparable to the other view graphs in absolute values, due to a change of microwave sources. Here,  $P_{N2}$  was chosen within the bistability window of neuron **N2**, and  $P_{N1}$  was chosen large enough to trigger **N2**. The resulting BLS-intensity shows the sharp trigger pulse, followed by the activated neuron signal. The emission of **N2** after triggering is visible in both positions, however, the emission in the forward direction (P1) is significantly stronger compared to the backward direction (P2). I.e., the emission is strongly non-reciprocal, as it often happens for the Damon-Eshbach geometry due to chirality of the magnetization precession and the excitation field [3].

## References

- [1] Heinz, B. *et al.* Long-range spin-wave propagation in transversely magnetized nano-scaled conduits. *Applied Physics Letters* **118**, 132406 (2021). URL <https://doi.org/10.1063/5.0045570>.
- [2] Breitbach, D. *et al.* Nonlinear erasing of propagating spin-wave pulses in thin-film Ga:YIG. *Applied Physics Letters* **124**, 092405 (2024). URL <https://doi.org/10.1063/5.0189648>.
- [3] Schneider, T., Serga, A. A., Neumann, T., Hillebrands, B. & Kostylev, M. P. Phase reciprocity of spin-wave excitation by a microstrip antenna. *Phys. Rev. B* **77**, 214411 (2008). URL <https://doi.org/10.1103/PhysRevB.77.214411>.
